# Supplementary material for: Coherence properties of shallow donor qubits in ZnO
Source: arXiv:1802.03483 ancillary file (2018-05-23)
Supplement: Supplementary file 1 [file supplementary.pdf]

# Supplementary information: Coherence properties of shallow donor qubits in ZnO

Xiayu Linpeng<sup>1</sup>, Maria L. K. Viitaniemi<sup>1</sup>, Aswin Vishnuradhan<sup>2</sup>, Y. Kozuka<sup>2,3</sup>, Cameron Johnson<sup>4</sup>, M. Kawasaki<sup>2</sup>, and Kai-Mei C. Fu<sup>1,5</sup>

<sup>1</sup>Department of Physics, University of Washington, Seattle, Washington 98195, USA

<sup>2</sup>Department of Applied Physics and Quantum-Phase Electronics Center (QPEC), University of Tokyo, Tokyo 113-8656, Japan

<sup>3</sup>JST, PRESTO, Kawaguchi, Saitama 332-0012, Japan

<sup>4</sup>Department of Physics, University of Oregon, Eugene, Oregon 97403, USA

<sup>5</sup>Department of Electrical Engineering, University of Washington, Seattle, Washington 98195, USA

## 1 Sample description and donor line identification

Experiments were carried out on a 0.7  $\mu\text{m}$  ZnO epitaxial film grown on a 360  $\mu\text{m}$ -thick ZnO substrate (Tokyo Denpa Co.). The total donor concentration is orders of magnitude higher in the substrate than in the epitaxial layer. As a result of the 1  $\mu\text{m}$  scale spot size, the signal collected is dominated by the substrate photoluminescence; therefore, in the main text we solely describe our sample as the substrate. Figure S1 shows a typical photoluminescence spectrum from the ZnO sample. The PL peaks are identified according to the assignments in Meyer et al. [1]. Measurements were performed on the two main donor peaks  $I_8$  and  $I_6$  corresponding to Ga and Al donors respectively. These lines result from the recombination of the  $\text{D}^0\text{X}$  excitons to the hydrogenic  $\text{D}^0$  1s state. The peaks around 3.32 eV are the two electron satellites (TES) of the Ga and Al  $\text{D}^0\text{X}$  transitions. The TES transitions correspond to the recombination of  $\text{D}^0\text{X}$  excitons to the  $\text{D}^0$  2s and 2p states [1]. Enhancement of the TES peaks is observed with resonant excitation of the main  $\text{D}^0\text{X}$  lines (Fig. S2).

The peak around 3.376 eV, labeled FX, is the free exciton line [1]. The origin of the band between the free exciton and the main donor lines is unknown and labeled “?”. This band’s shape and intensity are position dependent. The small peak at 3.333 eV is assigned to the Y line and is due to excitons bound to local defects (e.g. dislocations) [1].

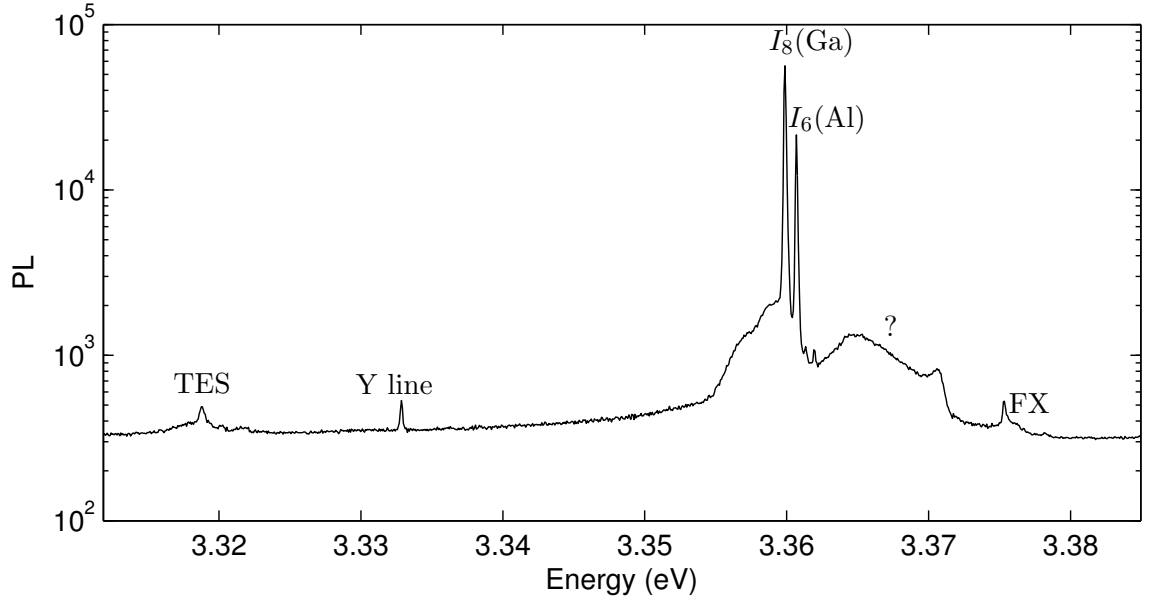

Fig. S1: Log-scale photoluminescence spectra of the ZnO sample at 0 T, 1.5 K. Excitation laser is at  $\sim 3.4$  eV and  $\sim 170$  nW with a laser spot size of  $1 \mu\text{m}$ .

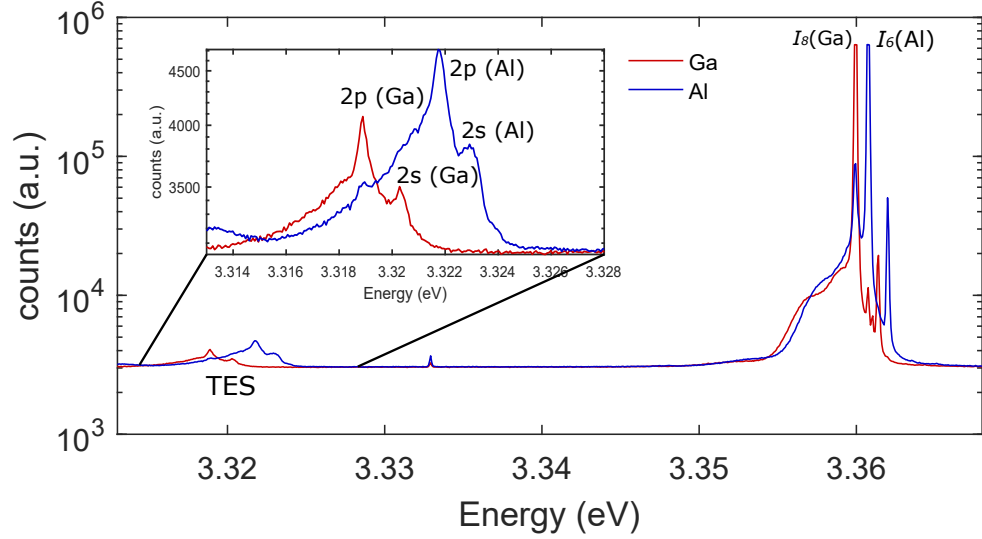

Fig. S2: Log-scale resonant photoluminescence spectra of the ZnO sample at 0 T, 1.5 K. Excitation laser is resonantly exciting the Ga (red) or Al (blue) main donor-bound exciton transition. The inset shows the enhancement of the two-electron satellite peaks.

## 2 Selection rules

From the  $\Gamma_7$  symmetry of the top valence band and the s-orbital nature of the conduction band electron [2,3,4], four optical transitions are allowed, two with  $\sigma^\pm$  polarization and two with  $\hat{z}$  polarization (Fig. S7(a)). We experimentally determine the branching ratio between the  $\sigma^\pm$  and  $\hat{z}$  transitions by comparing the intensity of H and V polarized spectra in Voigt geometry (Fig. 1(b) in the main text). The intensity ratio between H and V is 1.2, which gives the ratio of the dipole matrix elements for  $\sigma^\pm$  and  $\hat{z}$  transitions to be  $\mu_{\sigma^\pm} : \mu_{\hat{z}} = \sqrt{2} : \sqrt{1.2}$ . This also determines the parameter  $q_7 = 0.61$  in the  $k \cdot p$  theory for ZnO [4] and thus the hole wave function for the top valence band:

$$|\Gamma_7, \uparrow\rangle = \sqrt{1 - q_7^2} \left| \frac{\hat{x} + i\hat{y}}{\sqrt{2}}, \downarrow \right\rangle - q_7 |\hat{z}, \uparrow\rangle = 0.79 \left| \frac{\hat{x} + i\hat{y}}{\sqrt{2}}, \downarrow \right\rangle - 0.61 |\hat{z}, \uparrow\rangle \quad (\text{S1})$$

$$|\Gamma_7, \downarrow\rangle = -\sqrt{1 - q_7^2} \left| \frac{\hat{x} - i\hat{y}}{\sqrt{2}}, \uparrow \right\rangle - q_7 |\hat{z}, \downarrow\rangle = -0.79 \left| \frac{\hat{x} - i\hat{y}}{\sqrt{2}}, \uparrow \right\rangle - 0.61 |\hat{z}, \downarrow\rangle \quad (\text{S2})$$

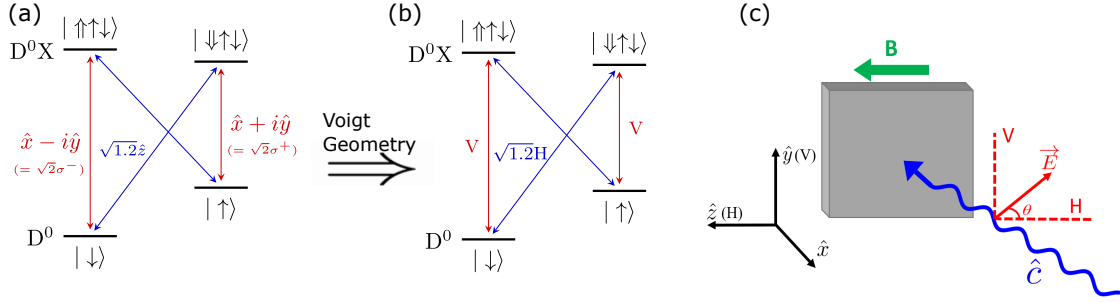

Fig. S3: (a) Optical selection rules determined by experimental data. (b) Selection rules in Voigt geometry. (c) The schematic of the Voigt geometry.  $B$  is the magnetic field.  $\hat{c}$  is the light propagation direction.  $\vec{E}$  shows the polarization direction.  $\theta$  is the angle between  $\vec{E}$  and  $H$ .

### 3 Effective 2-level Hamiltonian

The 4-level Hamiltonian describing our optical coherent spin control is given by

$$H = \begin{pmatrix} 0 & 0 & -\Omega_{13}(t)/2 - \Omega_{14}(t)/2 \\ 0 & \omega_e & -\Omega_{23}(t)/2 - \Omega_{24}(t)/2 \\ -\Omega_{13}^*(t)/2 - \Omega_{23}^*(t)/2 & \Delta & 0 \\ -\Omega_{14}^*(t)/2 - \Omega_{24}^*(t)/2 & 0 & \Delta + \omega_h \end{pmatrix} \quad (\text{S3})$$

$\omega_e(\omega_h)$  is the energy of the electron (hole) Zeeman splitting.  $\Delta$  is the red detuning between the ultra-fast laser and the transition  $|\downarrow\rangle \Leftrightarrow |\downarrow\uparrow\downarrow\rangle$ .  $\Omega_{ij}(t) = \vec{\mu}_{ij} \cdot \vec{E}(t)/\hbar$  is the product of the electric field and the dipole matrix element of transition  $|i\rangle \Leftrightarrow |j\rangle$  ( $i = 1, 2, 3, 4$  corresponding to states  $|\downarrow\rangle, |\uparrow\rangle, |\downarrow\uparrow\downarrow\rangle, |\uparrow\uparrow\downarrow\rangle$ ).

Reducing this 4-level Hamiltonian to an effective 2-level model is helpful for gaining intuition about population dynamics. A state  $|\Psi(t)\rangle = a_1(t)|\downarrow\rangle + a_2(t)|\uparrow\rangle + a_3(t)|\downarrow\uparrow\downarrow\rangle + a_4(t)|\uparrow\uparrow\downarrow\rangle$  will evolve according to

$$\frac{d|\Psi(t)\rangle}{dt} = -iH(t)|\Psi(t)\rangle. \quad (\text{S4})$$

The equations of motion for the coefficients can be written as

$$a_3\Omega_{13} + a_4\Omega_{14} = \dot{a}_1 \quad (\text{S5})$$

$$a_2\omega_e + a_3\Omega_{23} + a_4\Omega_{24} = \dot{a}_2 \quad (\text{S6})$$

$$a_1\Omega_{13}^* + a_2\Omega_{23}^* + a_3\Delta = \dot{a}_3 \quad (\text{S7})$$

$$a_1\Omega_{14}^* + a_2\Omega_{24}^* + a_4(\Delta + \omega_h) = \dot{a}_4 \quad (\text{S8})$$

in which  $\Omega_{ij}(t)$  and  $a_i(t)$  are time dependent.

If the pulse is far detuned from the donor-bound exciton transition energy, then  $\dot{a}_3 \ll a_3\Delta$  and  $\dot{a}_4 \ll a_4\Delta$ . By setting  $\dot{a}_3$  and  $\dot{a}_4$  to zero in Eqs. S7 and S8, we find

$$a_3 = -\frac{\Omega_{13}^*}{\Delta}a_1 - \frac{\Omega_{23}^*}{\Delta}a_2 \quad (\text{S9})$$

$$a_4 = -\frac{\Omega_{14}^*}{\omega_h + \Delta}a_1 - \frac{\Omega_{24}^*}{\omega_h + \Delta}a_2 \quad (\text{S10})$$

Inserting Eqs. S9 and S10 back into Eqs. S5 and S6 yields the effective 2-level Hamiltonian

$$H_{\text{eff}}(t) = \begin{pmatrix} -\frac{|\Omega_{31}(t)|^2}{4\Delta} - \frac{|\Omega_{41}(t)|^2}{4(\Delta + \omega_h)} & 0 \\ 0 & -\frac{|\Omega_{32}(t)|^2}{4\Delta} - \frac{|\Omega_{42}(t)|^2}{4(\Delta + \omega_h)} \end{pmatrix} + \begin{pmatrix} 0 & \frac{-\Omega_{\text{eff}}(t)}{2}e^{i\omega_e t} \\ \frac{-\Omega_{\text{eff}}^*(t)}{2}e^{-i\omega_e t} & 0 \end{pmatrix} \quad (\text{S11})$$

where  $\Omega_{\text{eff}}(t) = \frac{\Omega_{13}(t)\Omega_{23}^*(t)}{2\Delta} + \frac{\Omega_{14}(t)\Omega_{24}^*(t)}{2(\Delta + \omega_h)}$  is the effective Rabi frequency.

As explained in Sec. 5, we have experimentally set all  $\Omega_{ij}(t) = \Omega_R(t)$ . In this limit, the first term in  $H_{\text{eff}}$  is proportional to the identity and  $\Omega_{\text{eff}}(t)$  is reduced to  $\Omega_{\text{eff}}^{\text{exp}}(t)$ . This allows us to write

$$H_{\text{eff}}^{\text{exp}}(t) = \begin{pmatrix} 0 & \frac{-\Omega_{\text{eff}}^{\text{exp}}(t)}{2}e^{i\omega_e t} \\ \frac{-\Omega_{\text{eff}}^{\text{exp}*}(t)}{2}e^{-i\omega_e t} & 0 \end{pmatrix} \quad (\text{S12})$$

where  $\Omega_{\text{eff}}^{\text{exp}}(t) = \frac{|\Omega_R|^2}{2}(\frac{1}{\Delta} + \frac{1}{(\Delta + \omega_h)})$ .

To estimate the error in  $H_{\text{eff}}$ , simulations of a single-pulse experiment were done using both  $H_{\text{eff}}$  and the full 4-level Hamiltonian,  $H$ . For the data shown in Fig. 3 of the main text, the red detuning of the pulsed laser ( $\Delta/2\pi$ ) is 3.57 THz. For this laser detuning and for small pulse angles,  $H_{\text{eff}}$  and  $H_{4\text{lvl}}$  match well (Fig. S4). We find only a 1.7% difference in the Rabi frequency required for a  $\pi$  rotation. However, this model does not account for dephasing nor relaxation. Therefore for quantitative analysis, a 4-level model is used (Sec. 4).

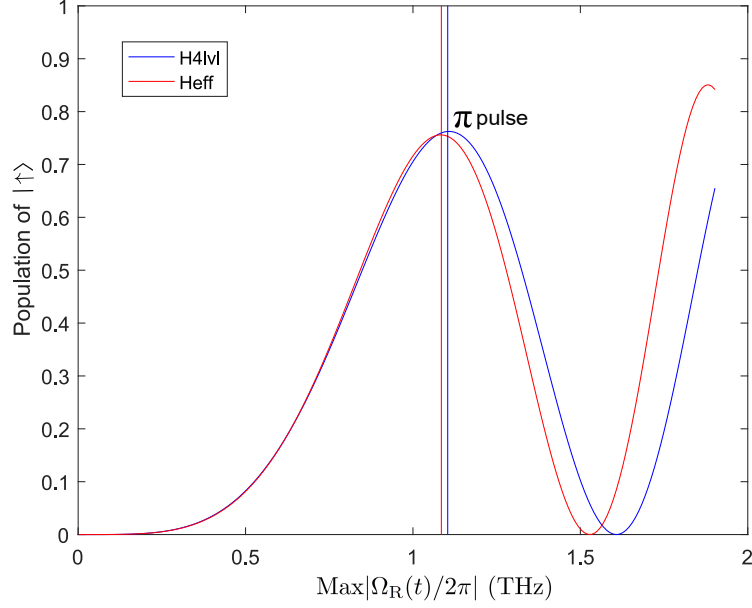

Fig. S4: Simulation results for the population of the  $|\uparrow\rangle$  state as a function of the Rabi frequency ( $\Omega_R$ , Sec. 5) after a single pulse. The laser detuning is 3.57 THz. The population is simulated using the effective Hamiltonian (red) and the 4-level Hamiltonian (blue).

## 4 Master Equation and Simulation Parameters

To simulate the dynamics of our system, we use a 4-level density matrix master equation

$$\partial\rho/\partial t = -i[H, \rho] + L(\rho), \quad (\text{S13})$$

where  $\rho$  is a 4-level density matrix,  $H$  is the Hamiltonian of our system (Eq. S3), and  $L(\rho)$  is the Lindblad operator describing decoherence processes (Eq. S14).

$$L(\rho) = \begin{pmatrix} -\Gamma_{12}\rho_{11} + \Gamma_{21}\rho_{22} + \Gamma_{31}\rho_{33} + \Gamma_{41}\rho_{44} & -(\frac{\Gamma_{12}+\Gamma_{21}}{2} + \gamma_{12})\rho_{12} & & & \\ -(\frac{\Gamma_{21}+\Gamma_{12}}{2} + \gamma_{12})\rho_{21} & \Gamma_{12}\rho_{11} - \Gamma_{21}\rho_{22} + \Gamma_{32}\rho_{33} + \Gamma_{42}\rho_{44} & & & \\ -(\frac{\Gamma_{31}+\Gamma_{32}+\Gamma_{34}+\Gamma_{12}}{2} + \gamma_{13})\rho_{31} & -(\frac{\Gamma_{31}+\Gamma_{32}+\Gamma_{34}+\Gamma_{21}}{2} + \gamma_{23})\rho_{32} & & & \\ -(\frac{\Gamma_{41}+\Gamma_{42}+\Gamma_{43}+\Gamma_{12}}{2} + \gamma_{14})\rho_{41} & -(\frac{\Gamma_{41}+\Gamma_{42}+\Gamma_{43}+\Gamma_{21}}{2} + \gamma_{24})\rho_{42} & & & \\ & -(\frac{\Gamma_{12}+\Gamma_{31}+\Gamma_{32}+\Gamma_{34}}{2} + \gamma_{13})\rho_{13} & -(\frac{\Gamma_{12}+\Gamma_{41}+\Gamma_{42}+\Gamma_{43}}{2} + \gamma_{14})\rho_{14} & & \\ & -(\frac{\Gamma_{21}+\Gamma_{31}+\Gamma_{32}+\Gamma_{34}}{2} + \gamma_{23})\rho_{23} & -(\frac{\Gamma_{21}+\Gamma_{41}+\Gamma_{42}+\Gamma_{43}}{2} + \gamma_{24})\rho_{24} & & \\ & -(\Gamma_{31} + \Gamma_{32} + \Gamma_{34})\rho_{33} + \Gamma_{43}\rho_{44} & -(\frac{\Gamma_{31}+\Gamma_{32}+\Gamma_{34}+\Gamma_{41}+\Gamma_{42}+\Gamma_{43}}{2})\rho_{34} & & \\ & -(\frac{\Gamma_{41}+\Gamma_{42}+\Gamma_{43}+\Gamma_{31}+\Gamma_{32}+\Gamma_{34}}{2})\rho_{43} & -(\Gamma_{41} + \Gamma_{42} + \Gamma_{43})\rho_{44} + \Gamma_{34}\rho_{33} & & \end{pmatrix} \quad (\text{S14})$$

$\Gamma_{ij}$  is the population relaxation rate from  $|i\rangle \rightarrow |j\rangle$  and  $\gamma_{ij}$  is the rate of dephasing between  $|i\rangle \leftrightarrow |j\rangle$ .

As explained in Sec. 5, we have experimentally set all  $\Omega_{ij}(t) = \Omega_R(t)$ . We fit for the relationship between  $\Omega_R(t)$  and pulse energy using  $P = \alpha \cdot \max|\Omega_R(t)|^2$ , where  $P$  is the pulse energy,  $\alpha$  is a fit parameter, and  $\max|\Omega_R(t)|^2$  is the peak value of  $|\Omega_R(t)|^2$  where we have assumed a Gaussian time dependence. Autocorrelation measurements of the infrared laser pulse find a pulse width of 1.9 ps; however, after second harmonic generation where  $I_{UV}(2\omega) \propto I_{IR}^2(\omega)$ , we estimate that the ultra violet laser pulse is compressed to  $1.9/\sqrt{2}$  ps.

$\gamma_{13} = \gamma_{23} = \gamma_{14} = \gamma_{24} = \gamma$  is the dephasing between the excited states and the ground states. Due to laser-induced dephasing, we fit for  $\gamma = \beta_1\Omega_R(t) + \beta_2\Omega_R^2(t)$  where  $\beta_1$  and  $\beta_2$  are fit parameters.  $\Gamma_{31} = \Gamma_{42} = 0.38\Gamma_{\text{rad}}$  and  $\Gamma_{32} = \Gamma_{41} = 0.62\Gamma_{\text{rad}}$  are the radiative decay rates from the excited states to the ground states based on the selection rules in Fig. S7. We let  $\Gamma_{12} = \Gamma_{21} = \Gamma_{34} = \Gamma_{43} = 0$ , because these decay rates are slow compared to the other time scales in this system. Parameters used in the simulation in Fig. 3 of the main text are given in Table S1.

| Parameter             | Value                                               | Description                                                                                                 |
|-----------------------|-----------------------------------------------------|-------------------------------------------------------------------------------------------------------------|
| $\omega_e$            | $2\pi \times 138 \text{ GHz}^a$                     | ground state frequency splitting, $\omega_e = g_e \mu_B B / \hbar$                                          |
| $\omega_h$            | $2\pi \times 24 \text{ GHz}^a$                      | excited state frequency splitting, $\omega_h = g_h \mu_B B / \hbar$                                         |
| $\Delta$              | $2\pi \times 3570 \text{ GHz}^b$                    | detuning between pulsed laser and $ \downarrow\rangle \Leftrightarrow  \downarrow\uparrow\downarrow\rangle$ |
| $\Gamma_{\text{rad}}$ | $1 \text{ GHz} [5]$                                 | $1/T_{\text{rad}}$ , $T_{\text{rad}}$ is the radiative lifetime                                             |
| $\gamma_{12}$         | $5 \times 10^{-5} \text{ GHz}^c$                    | $1/T_2$                                                                                                     |
| $\alpha$              | $7.2 \times 10^{-6} \text{ pJ GHz}^{-2} \text{ }^d$ | $P = \alpha \cdot \max \Omega_R(t) ^2$                                                                      |
| $\beta_1$             | $6.6 \text{ }^d$                                    | $\gamma = \beta_1 \Omega_R + \beta_2 \Omega_R^2$                                                            |
| $\beta_2$             | $3.3 \times 10^{-3} \text{ GHz}^{-1} \text{ }^d$    | $\gamma = \beta_1 \Omega_R + \beta_2 \Omega_R^2$                                                            |

Table S1: Parameters used for the simulation in Fig. 3.

<sup>a</sup> Derived from the electron and hole g-factors,  $g_e$  and  $g_h$  respectively, measured using the data in Fig. 1c

<sup>b</sup> Experimental parameter

<sup>c</sup>  $T_2$  measured from the data in Fig. 4

<sup>d</sup> Fit from the data in Fig.3

## 5 Determination of optical pulse polarization

A half-wave plate controls both the angle of the control pulse polarization and the polarization of the collected photoluminescence. This angle is set such that  $\Omega_{13} = \Omega_{23} = \Omega_{14} = \Omega_{24} = \Omega_R$ . Figure S5(a) shows typical spectra of the Ga and Al transitions when exciting at 3.37 eV. Because of the transition linewidth and the spectrometer resolution, the  $|\uparrow\rangle_{\text{Ga}}$  peak includes both the  $|\uparrow\rangle \leftrightarrow |\downarrow\uparrow\downarrow\rangle$  and  $|\uparrow\rangle \leftrightarrow |\uparrow\uparrow\downarrow\rangle$  transitions. Changing the polarization of the collected photoluminescence from vertical to horizontal causes a shift in the  $|\uparrow\rangle_{\text{Ga}}$  peak from the  $|\uparrow\rangle \leftrightarrow |\downarrow\uparrow\downarrow\rangle$  to the  $|\uparrow\rangle \leftrightarrow |\uparrow\uparrow\downarrow\rangle$  transition energy. In other words, we select a polarization angle (Fig. S5) such that  $\Omega_{23}(t) = \vec{\mu}_{23} \cdot \vec{E}(t)/\hbar = \mu_{23}E(t)\cos\theta/\hbar$  and  $\Omega_{24}(t) = \vec{\mu}_{24} \cdot \vec{E}(t)/\hbar = \mu_{24}E(t)\sin\theta/\hbar$  equal each other. This allows us to set  $\Omega_{ij}(t) = \Omega_R(t)$  in our simulations.

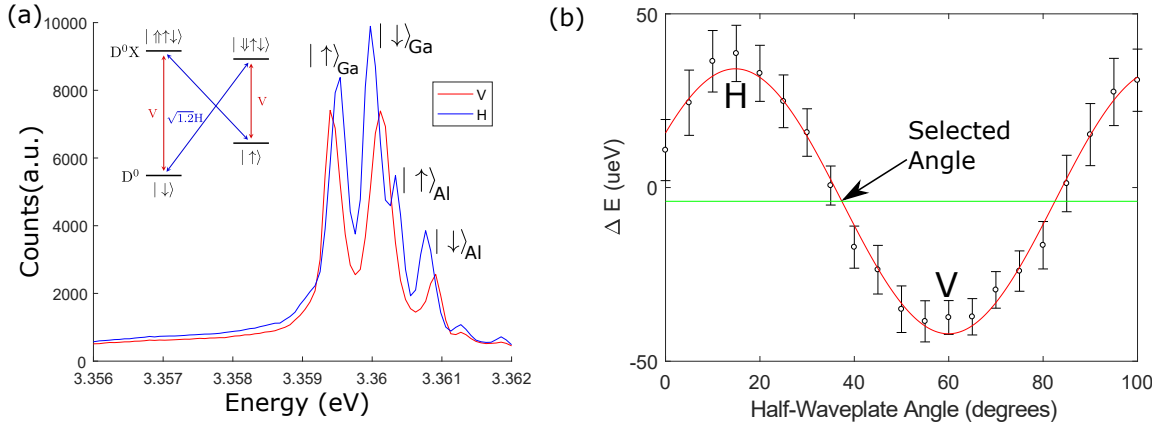

Fig. S5: (a) Typical spectra of vertically (red) and horizontally (blue) polarized photoluminescence at 5 T. Both spectra are excited with 3.37 eV. The inset shows the energy diagram and selection rules in Voigt geometry. (b) Change in the energy of the  $|\uparrow\rangle_{\text{Ga}}$  peak as a function of half-waveplate angle. Horizontal (H), vertical (V), and the selected angle are labeled.

## 6 Effect of the beam size on the power dependence of $P_{\uparrow}$ and $V$

In Fig. 3 of the main text, the fit using the 4-level master equation model underestimates the experimentally observed power dependence of Ramsey fringe amplitude  $V$ . We attribute this to the effect of small beam size, which leads to different spin rotation angles of donors in the collection spot. Figure S6 shows a simulation of this effect. In the “large beam” case, a single power model (solid lines in the figures) can fit the simulated experimental results (dots in the figures) well for both  $P_{\uparrow}$  and  $V$ . In the “small beam” case, though the power dependence of  $P_{\uparrow}$  fits well, the simulated experimental fringe amplitude  $V$  is higher than  $V$  fit using the single power model. This is consistent with the underestimation in the fit for experimental data in Fig. 3 of the main text.

It should be noted that the beam size written in the caption of Fig. 3 in the main text is the approximate size of the reflected beam on the sample surface. More accurately, the shape of the reflected beam is an oval (1.5  $\mu\text{m}$  in short axis and 3.5  $\mu\text{m}$  in long axis). Though the recorded beam size is larger than the collection spot (0.6  $\mu\text{m}$ ), the beam is focused inside the sample and the size of the focused beam is in the limit of “small beam” case.

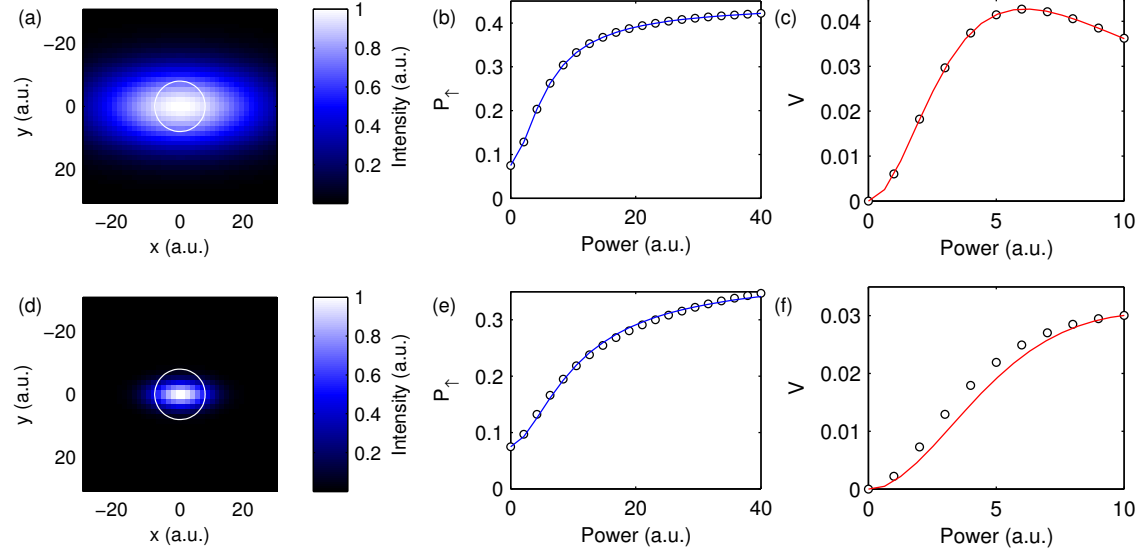

Fig. S6: (a) Comparison of the beam size and collection spot size in “large beam” case. The white circle in the middle shows the collection spot. The intensity of the 2D map represents the relative intensity of the pulse beam. (b)  $P_{\uparrow}$  as function of the power of the pulse. The dots are simulated experimental results by summing the different laser powers across the collection spot. The solid line is a fit using the master equation model assuming a single pulse power. (c)  $V$  as function of the power of the pulse. The dots are simulated experimental results by summing the different laser powers across the collection spot. The solid line is a fit using the master equation model assuming a single pulse power. The fit in **c** uses the same parameters in **b**. (d-f) The same as (a-c) but in the “small beam” case.

## 7 Estimation of the hyperfine field distribution

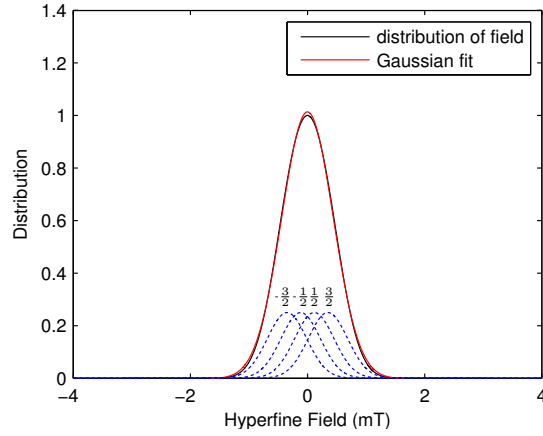

Fig. S7: The 4 dashed curves show the distribution of the hyperfine field with Ga in the four different nuclear spin states, i.e.  $m_{Ga} = \{\frac{3}{2}, \frac{1}{2}, -\frac{1}{2}, -\frac{3}{2}\}$ . The black line is the distribution of the hyperfine field combining the contributions from both Ga and  $^{67}\text{Zn}$ . In the combination, the nuclear spin states are assumed to be equally distributed in the 4 spin states as the nuclear splitting is much smaller than the thermal energy. The red curve is a fit using a Gaussian form  $e^{-B^2/\Delta_B^2}$ , where the dispersion  $\Delta_B$  is used to estimate  $T_2^*$  with  $T_2^* = \hbar/g_e\mu_B\Delta_B$ .

## References

1. B. K. Meyer, H. Alves, D. M. Hofmann, W. Kriegseis, D. Forster, F. Bertram, J. Christen, A. Hoffmann, M. Straßburg, M. Dworzak, U. Haboeck, and A. V. Rodina, “Bound exciton and donor-acceptor pair recombinations in ZnO,” *Physica Status Solidi (B) Basic Research*, vol. 241, no. 2, pp. 231–260, 2004.
2. M. R. Wagner, J.-H. Schulze, R. Kirste, M. Cobet, A. Hoffmann, C. Rauch, A. V. Rodina, B. K. Meyer, U. Röder, and K. Thonke, “Gamma<sub>7</sub> valence band symmetry related hole fine splitting of bound excitons in zno observed in magneto-optical studies,” *Phys. Rev. B*, vol. 80, p. 205203, 2009.
3. R. Laskowski and N. E. Christensen, “Ab initio calculation of excitons in ZnO,” *Physical Review B*, vol. 73, Jan. 2006.
4. L. C. Lew Yan Voon, M. Willatzen, M. Cardona, and N. E. Christensen, “Terms linear in k in the band structure of wurtzite-type semiconductors,” *Physical Review B*, vol. 53, pp. 10703–10714, Apr. 1996.
5. M. R. Wagner, G. Callsen, J. S. Reparaz, J. H. Schulze, R. Kirste, M. Cobet, I. A. Ostapenko, S. Rodt, C. Nenstiel, M. Kaiser, A. Hoffmann, A. V. Rodina, M. R. Phillips, S. Lautenschläger, S. Eisermann, and B. K. Meyer, “Bound excitons in ZnO: Structural defect complexes versus shallow impurity centers,” *Physical Review B - Condensed Matter and Materials Physics*, vol. 84, no. 3, pp. 1–18, 2011.
